# Supplementary material for: Janus Percolation in Anisotropic Limited-Degree Networks
Source: arXiv:2512.10566 ancillary file (2025-12-11)
Supplement: Supplementary file 1 [file janus_supplementary.pdf]

# Supplementary Material for: Janus Percolation in Anisotropic Limited-Degree Networks

Jacopo A. Garofalo,[1,*] Nuno A.M. Araújo,[2] Lucilla de Arcangelis,[1] Alessandro Sarracino,[3] and Eugenio Lippiello[1]

[1] *Department of Mathematics and Physics, University of Campania "Luigi Vanvitelli", Viale Lincoln 5, Caserta, 81100, Italy*
[2] *Centro de Física Teórica e Computacional, Faculdade de Ciências, Universidade de Lisboa, Campo Grande 016, Lisboa, 1749-016, Portugal*
[3] *Department of Engineering, University of Campania "Luigi Vanvitelli", Via Roma 29, Aversa, 81031, Italy*

(Dated: December 11, 2025)

## WEAKLY CONNECTED COMPONENTS AND ADDITIONAL MATERIAL ON STRONGLY CONNECTED COMPONENTS

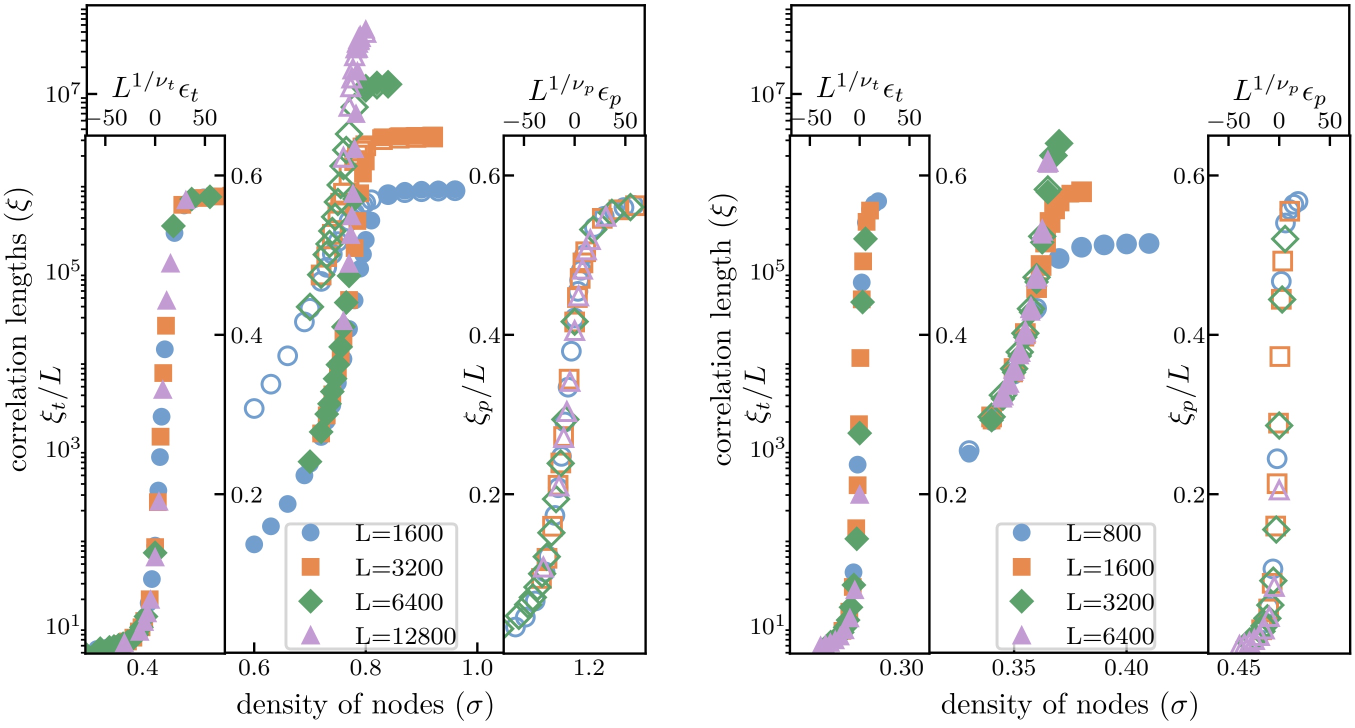


FIG. 1: **Finite-size scaling of correlation lengths for WCCs.** Filled and open symbols represent respectively correlation lengths measured along directions transverse ($\xi_t$) and parallel ($\xi_p$) to the preferential one . The left and right panels show the correlation lengths along the two axes and the respective insets are the data collapses obtained using the *Ansatz* in Eq. 2 of the main manuscript. Left panel shows results for $q = 1.01$, while the right one those for $q = 2$. Data collapses have been obtained with the following critical thresholds and exponents: $\nu_p = \nu_t = 4/3$, $\sigma_c(q = 1.01) = 0.78$, $\sigma_c(q = 2) = 0.365$. For the case $q = 2$, we can appreciate that the correlation lengths $\xi_p$ and $\xi_t$ are almost identical, which is expected when finding RP exponents. As for the case $q = 1.01$, even if there is a clear difference in $\xi_p$ and $\xi_t$ curves, which highlights anisotropy, the transitions along both still behave as RP.

---

* jacopoalexander.garofalo@unicampania.it

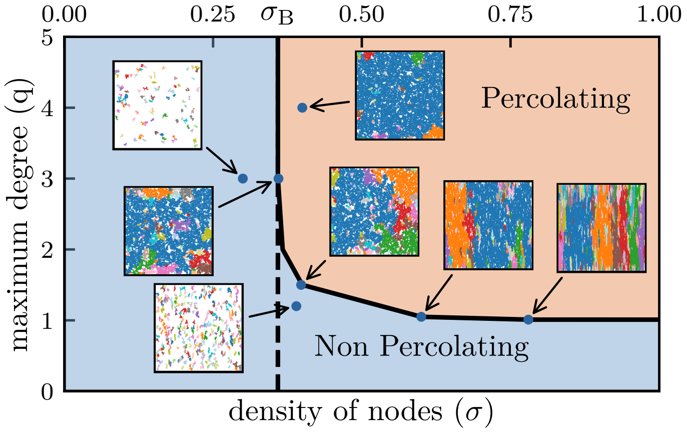


FIG. 2: **Two-parameter percolation diagram ($\sigma$,q) for WCCs**. Phase diagram of the WCCs in the $(\sigma, q)$ plane, where $\sigma$ is the node density and $q$ the maximum out-degree. The solid line marks the transition between the non-percolating and percolating phases, which is always a random percolation (RP) transition. Decreasing $q$, one finds that the percolation threshold $\sigma_c(q)$ goes from the one of the typical Boolean Model, $\sigma_B \simeq 0.359$, shown as the vertical dashed line, to diverging for $q \to 1$ from above. At $q = 1$ in fact we expect not to find critical behavior, as our model can be mapped into a branching process with branching ratio $b < 1$. Interestingly, for small $q$, even if we find highly anisotropic WCCs, as shown in the insets, they still only exhibit RP transitions, with simply a percolation thresholds that shifts towards higher densities. Insets show representative snapshots for a system of size $L = 1600$, where colors denote distinct SCCs; only components with size $M > 500$ are displayed.

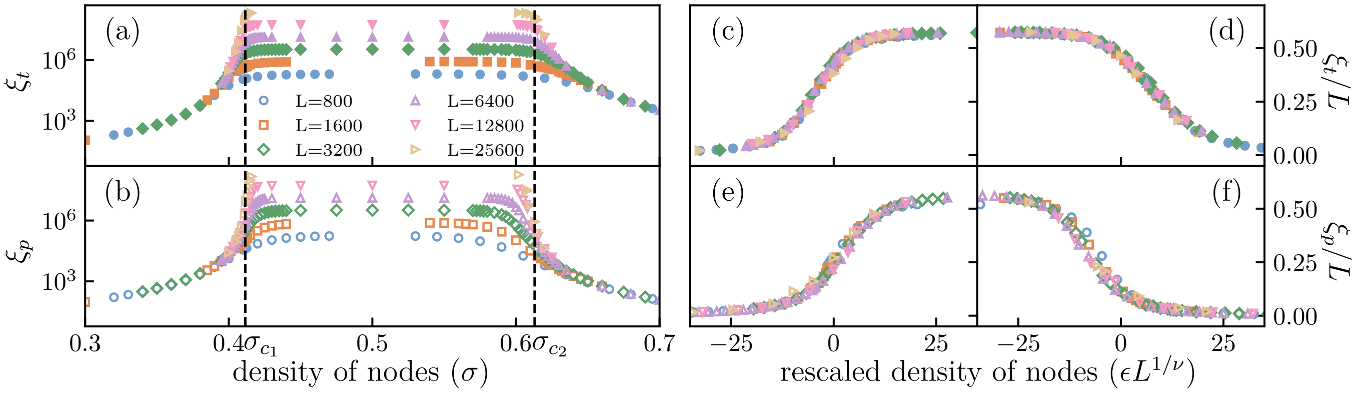


FIG. 3: **Finite-size scaling of correlation lengths for SCCs revealing mixed universality in both transitions.** Filled and open symbols represent correlation lengths measured along the directions transverse and parallel to the preferential one, respectively. Panels (a) and (b) show the raw correlation lengths for strongly connected components (SCCs) at $q = 5$, the vertical dashed lines are the thresholds for the first and second transition. The corresponding data collapses are presented in the right column: (c,d) are respectively the collapses for the first and second transition of panel (a), similarly (e,f) are those for data in panel (b). Collapses are obtained using the finite-size scaling *Ansatz* of Eq. 2 of the manuscript, with $\epsilon = (\sigma - \sigma_c)/\sigma_c$. The best data collapses are obtained using two slightly different values of the percolation thresholds, for the transverse and the perpendicular direction. We found for the transverse direction $\sigma^t_{c_1} = 0.411$ and $\sigma^t_{c_2} = 0.614$, while for the parallel one $\sigma^p_{c_1} = 0.414$ and $\sigma^p_{c_2} = 0.609$. Then as for the critical exponents, $\nu_t \simeq 1.734$ (directed percolation, DP) for the first transition on the transverse direction (panel (c)), and $\sigma_{c_2} \simeq 0.612$ with $\nu_t \approx 1.734$ (directed percolation, DP) for the second (panel (d)). Both transitions in the parallel direction are consistent with RP exponents, $\nu_{p_1} = \nu_{p_2} = \nu_r = 4/3$, (panels (g,h)).

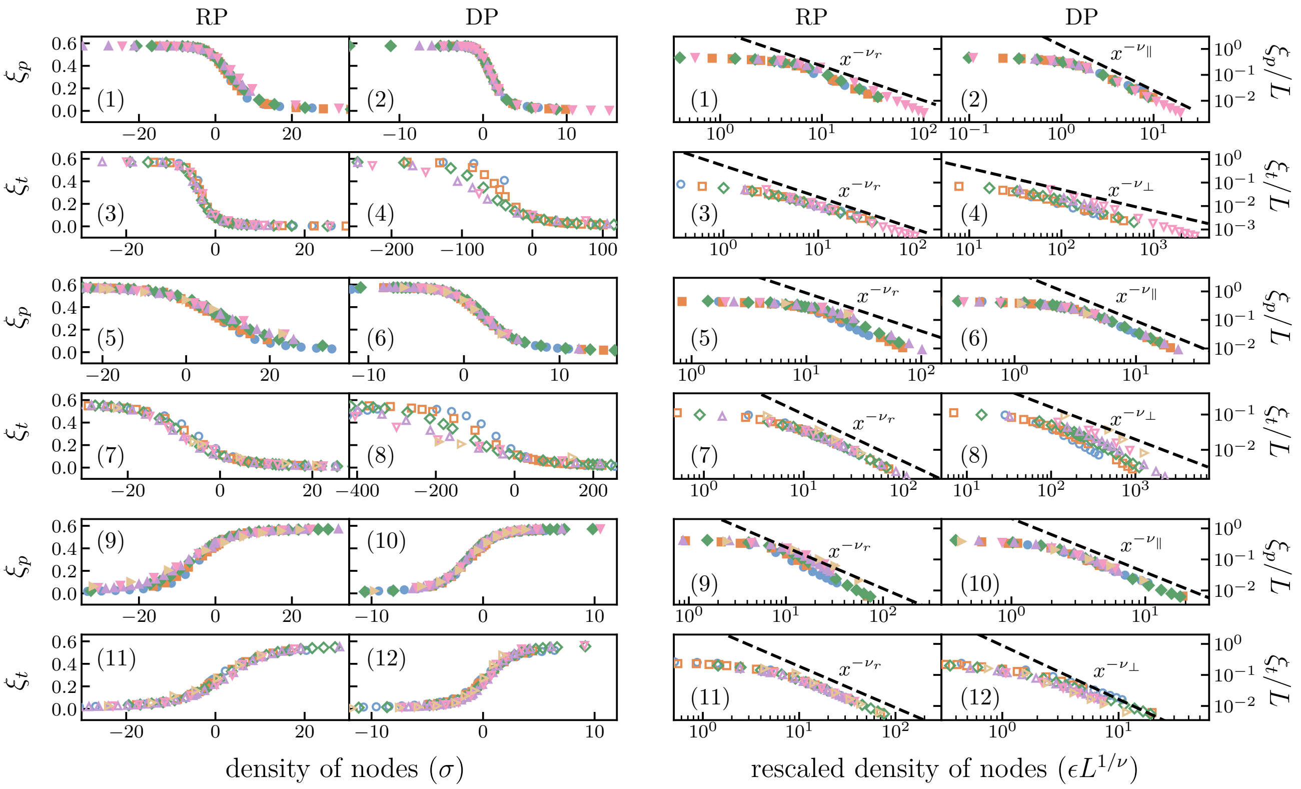

FIG. 4: **Comparison of the data collapses for SCCs obtained with exponents from different Universality Classes.** The panels show data collapses obtained following the general *Ansatz* in Eq. 2 of the main manuscript. Filled and empty symbols are used for correlation lengths along the transverse ($\xi_t$) and parallel $\xi_p$ directions respectively. The left panels show the data on linear scales, while the right panels display the same data on log–log axes, where the slope of the resulting straight lines allows a clearer discrimination of the critical exponents that best collapse the data. Each panel in the left column has a corresponding panel in the right column, and they share the same numbering. Panels (1-4) correspond to the second transition at $q = 7$, panels (5-8) to the second transition at $q = 5$, and panels (9-12) to the first transition at $q = 5$. For each block of four panels, the first two show the data collapse of $\xi_t$ using, respectively, the RP and DP exponents, while the following two panels display the rescaled $\xi_p$, again using the RP and DP exponents. Therefore, first and third columns of panels are data rescaled with RP exponents ($\nu_r = 4/3$), second and fourth columns instead with DP exponents. We identify with $\nu_r = 4/3$ the correlation length exponents of RP, while $\nu_\parallel \approx 1.734$ and $\nu_\perp \approx 1.097$ those for DP, along the parallel and transverse directions respectively, relative to the preferred axis. Note that, since in our model the clusters are elongated transversely to the preferential direction, in the scaling we try to use $\nu_\parallel$ on the $\xi_t$, and $\nu_\perp$ on the $\xi_p$.

TABLE I: Universality Classes of the transitions found for strongly connected components (SCCs) for different values of $q$.

| Maximum out-degree ($q$) | Direction | First transition | Second transition |
|---|---|---|---|
| $q < 6$ | transverse | DP | DP |
| | parallel | RP | RP |
| $q \geq 6$ | transverse | RP | DP |
| | parallel | RP | RP |
